# Supplementary material for: VCC-INFUSE: Towards Accurate and Efficient Selection of Unlabeled Examples in Semi-supervised Learning
Source: arXiv:2404.11947 source file (2024-04-21)
Supplement: Supplementary file 3 [file imagenet.tex]

\section{Experiment on ImageNet Dataset}
\label{imagenet}
\begin{table}[!h]
\centering
\caption{The accuracy of FixMatch, FlexMatch and their VCC versions on ImageNet-32 dataset.}
\label{table:imagenet}
\scalebox{0.9}{
\begin{tabular}{c|cc|cc}
\toprule
Method & FixMatch & w/VCC & FlexMatch & w/VCC \\ \hline
Acc(\%) & 32.06 & \textbf{36.53} & 36.89 & \textbf{39.21}\\
\bottomrule
\end{tabular}}
\end{table}
Apart from experiments on different dataset like CIFAR10, we also follow previous works to conduct a verification experiment on larger ImageNet dataset, which is more difficult. We carry out trials on ImageNet-32 based on FixMatch and FlexMatch with 100 labels per class (less than 8\%). The results are shown at Table \ref{table:imagenet}.

With VCC plugged in, both FixMatch and FlexMatch achieve better performance in accuracy. An improvement of 4.47\% on accuracy can be witnessed on FixMatch. Besides, FlexMatch also achieves 39.21\% with VCC. These results show consistent provement as in revious experiments and also further prove the effectiveness of our method.
